# Supplementary material for: Huddle test measurement of a near Johnson noise limited geophone
Source: arXiv:1711.05439 ancillary file (2017-11-15)
Supplement: Supplementary file 1 [file Supplementarymaterial1.pdf]

# Huddle test measurement of a near Johnson noise limited geophone

R. Kirchhoff,[1, a)] C. M. Mow-Lowry,[2] V. B. Adya,[3] G. Bergmann,[1] S. Cooper,[2] M. M. Hanke,[1] P. Koch,[1] S. M. Köhlenbeck,[1] J. Lehmann,[1] P. Oppermann,[1] J. Wöhler,[1] D. S. Wu,[1] H. Lück,[1, 3] and K. A. Strain[1, 4]

[1)] *Albert-Einstein-Institute / Max-Planck-Institute for Gravitational Physics, D-30167 Hanover, Germany*
[2)] *University of Birmingham, Birmingham B15 2TT, United Kingdom*
[3)] *Leibniz Universität Hannover, D-30167 Hanover, Germany*
[4)] *SUPA, School of Physics and Astronomy, University of Glasgow, G12 8QQ, United Kingdom*

(Dated: 17 August 2017)

## Supplementary material

In this supplementary material the amplifier circuits for the L-22D geophones and the L-4C geophones are pictured.

[a)] Electronic mail: robin.kirchhoff@aei.mpg.de

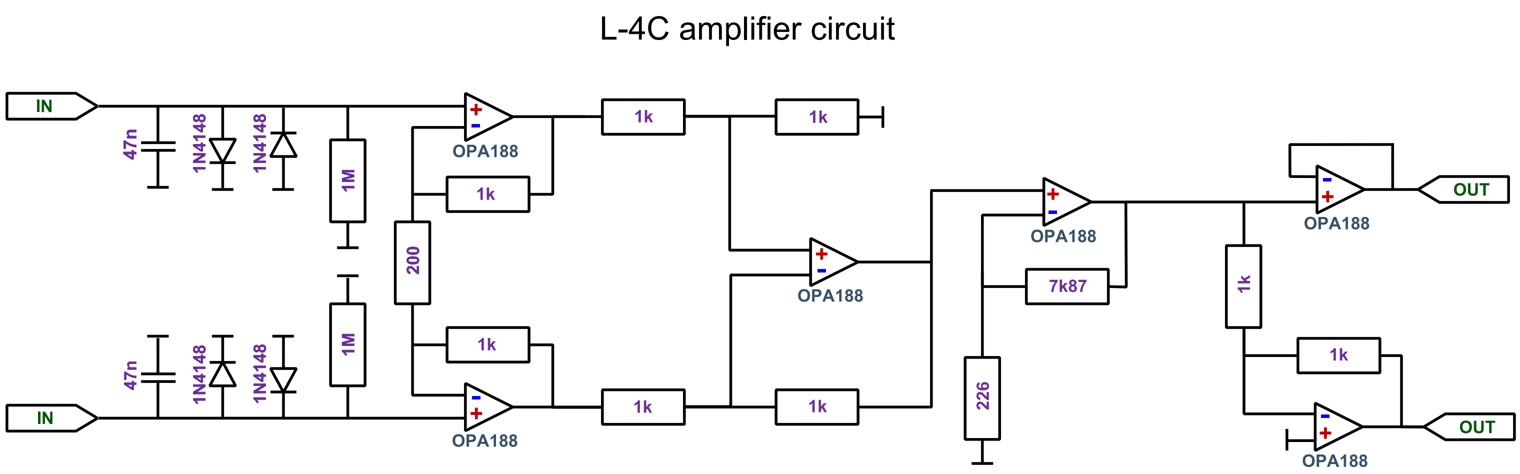


FIG. 1. Amplifier circuit for the L-4C geophones. The circuit consists of three stages, a differential input stage, a gain stage and a differential output stage all based on the low noise operational amplifier OPA188.

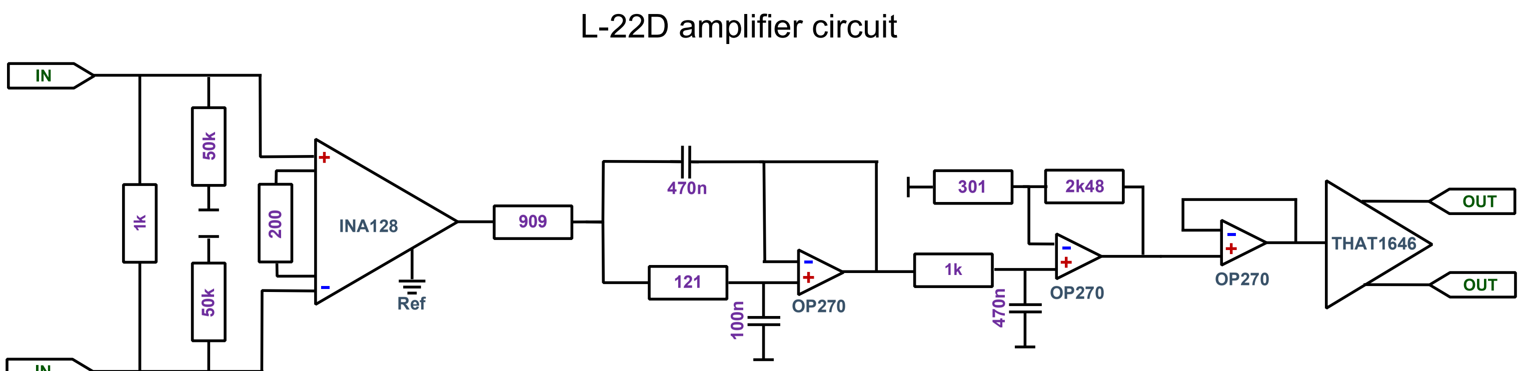


FIG. 2. Amplifier circuit for the L-22D geophones. The circuit consists of a differential input stage utilizing the instrument amplifier INA128, different gain and buffering stages utilizing the OP270 and a differential output stage utilizing the differential amplifier THAT1646.
