# Supplementary material for: Huddle test measurement of a near Johnson noise limited geophone
Source: arXiv:1711.05439 ancillary file (2017-11-15)
Supplement: Supplementary file 2 [file Supplementarymaterial2.pdf]

```
function [ sig_asd, resid_asd, freq, fit_vect, cor ] = mccs2(
signal_time_series, ref_time_series , Ts, smooth_width, poly_fit_terms,
win_pointer, varargin)
%mccs2  Mulit-Channel Coherent Subtraction, 'optimally' remove a several ref
channels from a data stream.
%
%  Based on the specExplain function by Wensheng Hua; removes the
%  correlated components of the reference channels from the signal channel
%  Part of the asd2, tfe2, coh2 family.
%
%  [ sig_asd, residual_asd, freq, fit_vect] = mccs2( signal_time_series,
ref_time_series, Ts, smooth_width, poly_fit_terms, win_pointer)
%
%   - required inputs-
%  signal_time_series   time series to analyze,
%  ref_time_series      set of referece time series. Each channel must be the
same
%                        length as signal_time_series. (presumably sampled
simultaneously).
%
%  Ts              the sampling time in seconds (time between consecutive
samples)
%   - optional inputs -
%  smooth_width   number of raw fft bins to average across (default is 9) -
%                 this is like the number of averages. MUST BE ODD!
%  poly_fit_terms order of polynomial to be removed from the data,
%                 (we use polyfit) 0 = DC, 1 = DC and best fit line,
%                 2 = DC, line, and parabola, etc.  (default is 1)
%  win_pointer    pointer to the built-in window, (default is @hann,
'periodic')
%                   see 'help window' for more information on windows
%
%   - outputs -
%  sig_asd   Amplitude Spectral Density of the signal channel.
%            should be the same as asd2, except sometimes the asd2 has 1 more
freq point.
%  residual_asd  ASD of the signal channel after an optimal subtraction of
%             the reference channel.
%      e.g. if signal_time_series is a horizontal ground T240 and
%        ref_time_series is a ground rotation sensor, the resid_asd is
%        the ground sensor spectrum with the rotation removed.
%  freq    freq vector for sig_asd and residual_asd
%       Note - the final bin width will be
%       BW = number of averages / length of time series in sec.
%       e.g. a 1000 sec time series with 50 averages will return a
%       freq with bin width (freq resolution) of 50/(1000 sec) = 50 mHz
%  fit_vect  like a transfer function - the best-fit coefficient for each
%       frequency bin. it is complex. unlike a 'real' TF, there is no
%       restriction on the relationships for magnitude and phase from one
%       frequncy bin to the next.
%
%  e.g. for data sets called gnd_T240_X and gnd_BRS_RY,
%       which were saved at 1/512 time steps, you might type:
%    [gnd_T240_X_asd, gnd_T240_tiltcorrected_asd, freq, fit_vect] = ...
%           sccs2(gnd_T240_X, gnd_BRS_RY, 1/512, 9, 1, @hann);
%
%   You can also call sccs with only the first 3, 4, or  5 inputs, e.g.
```

```
%    [asd_sig, asd_resid, freq, fit] = sccs2(signal_time_series,
time_series2, Ts);
%    [asd_sig, asd_resid, freq, fit] = sccs2(signal_time_series,
time_series2, Ts, smooth_width);
%    [asd_sig, asd_resid, freq, fit] = sccs2(signal_time_series,
time_series2, Ts, smooth_width, poly_fit_terms);
%
%    You can call mccs2 with [] as the inputs for:
%       smooth_width,  poly_fit_terms, and win_pointer, e.g.
%
%    [asd_sig, asd_resid, freq, fit] = mccs2(time_series1, time_series2, Ts,
[], poly_fit_terms);
%
%    inputs which are [] or not included will be set to the default values:
%    smooth_width = 9, poly_fit_terms = 1, and win_pointer = @hann.
%
%   The first bin (freq = 0) is set to 0, and not calculated.
%   since we remove means, and add windows, this bin is junk, anyways.
%
%  Idea - take the fft of the signal and ref, break it into bins,
%  for each bin, do a best-fit removal of the ref from the signal.
%
%  note the statistal correction factor of
%  sqrt(1-ref_channels/smooth_width) has been applied.
%
%   see also tfe2, coh2, and asd2
%
%    BTL wrote asd2.m on Sept 27, 2012
%    and adapted it to sccs2.m on Oct 24, 2014
%

% steps are:
% 0) Check inputs, set defaults for non-existant or empty values.
% 1) detrend each time series
%     by default we remove a 1st order poly, i.e. mean and slope,
%     but the user can pick something else.
% 2) apply a single window to each time series,
%    periodic hann window by default (0 at one end, one point away from 0 at
the
%    other), user can pick. The window is normalized so that the mean POWER
%    (amplitude squared) of the window is 1.
% 3) make a for loop through the specExplain steps
% 3b) apply the statical correction factor.
% 4) make the freq vector

%% 0) check inputs

debugging = false;

if ~exist('signal_time_series','var') || isempty(signal_time_series)
    error('input signal_time_series not defined, see help mccs2')
end

if ~exist('ref_time_series','var') || isempty(ref_time_series)
    error('input ref_time_series not defined, see help mccs2')
end
```

```
% make the input into a column vector
[rows, cols1] = size(signal_time_series);
if (rows > 1) && (cols1 > 1)
    error('input time series 1 must be a vector')
end
if (cols1 > 1)     % input1 is a row vector, change it
    if debugging; disp('flip sig chan'); end
    signal_time_series = signal_time_series.';  % flip it
end


orig_points       = length(signal_time_series);

% make sure this is size(dat_points,chans)
% choices are input is
% size is (orig_points, N) -> do nothing
% (N, orig_points) -> flip it,
% (something else) -> error


[rows2, cols2] = size(ref_time_series);
if (rows2 == orig_points)
    % ref is series of column vectors - do nothing
    if debugging; disp('no flip ref chan'); end
    ref_chans = cols2;
elseif (cols2 == orig_points)
    if debugging; disp('flip ref chan'); end
    ref_time_series = ref_time_series.';  % flip it
    ref_chans = rows2;
else
    error('MCCS:BadInputSize',...
        ['ref chans should be a matrix - one column per reference time
series\n',...
        'All ref channels must be the same length\n',...
        'as the signal channel']);
end


if ~exist('Ts','var') || isempty(Ts)
    error('input Ts not defined, see help mccs2')
end


if ~exist('smooth_width','var') || isempty(smooth_width)
    smooth_width = 9;
end



if smooth_width <1
    error('smooth width must be >= 1')
end
```

```
if (smooth_width ~= (1 + 2*round((smooth_width-1)/2)))  % is smooth_width
odd?
    error('the smooth_width param must be an odd integer');
end


if ~exist('poly_fit_terms','var') || isempty(poly_fit_terms)
    poly_fit_terms = 1;
end


if ~exist('win_pointer','var') || isempty(win_pointer)
    win_pointer = @hann;
end


if isempty(varargin)  % could add checking and processing here.
    user_window_args = false;
else
    user_window_args = true;
end


%% 1) detrend the data

time = Ts * (1:orig_points)';


 if orig_points < 1e4
    step = 1;
  elseif orig_points < 1e5
    step = 10;
  elseif orig_points < 1e6
    step = 100;
  elseif orig_points < 1e7
    step = 1E3;
  elseif  orig_points < 1e8
    step = 1E4;
   else
    step = 1E5;
    cprintf([1 0 0.5],'You are insane, how much data do you think that we can
handle?\n')
 end


fit_coefs1      = polyfit(time(1:step:end), signal_time_series(1:step:end),
poly_fit_terms);
detrended_data1 = signal_time_series - polyval(fit_coefs1, time);

detrend_ref = zeros(size(ref_time_series));
for ii = 1:ref_chans  % detrend each ref channel
    fit_coefs2       = polyfit(time(1:step:end),
ref_time_series(1:step:end,ii), poly_fit_terms);
```

```
    detrend_ref(:,ii) = ref_time_series(:,ii) - polyval(fit_coefs2, time);
end

if debugging == true
    figure
    pp = plot(time, signal_time_series, 'b', time, detrended_data1, 'm');
    set(pp,'LineWidth',2)
    title('orig data 1 vs. detrended data 1')
    xlabel('time (sec)')
    ylabel('mag')
    legend('orig data', 'detrended data')
    grid on

    figure
    for ii = 1:ref_chans
        subplot(ref_chans,1,ii)
        pp = plot(time, ref_time_series(:,ii), 'b', ...
            time, detrend_ref(:,ii), 'm');
        set(pp,'LineWidth',2)
        title(['Orig ref vs Detrended ref, chan ',num2str(ii)])
        xlabel('time (sec)')
        ylabel('mag')
        legend('orig data', 'detrended data')
        grid on
        FillPage('t')
        IDfig
    end

    disp(' ')
    disp([' using a ',num2str(poly_fit_terms),' order fit'])
    disp('poly fit coefs for time series 1 are: ')
    disp(fit_coefs1)
    %disp('poly fit coefs for time series 2 are: ')
    %disp(fit_coefs2)

end

clear  sig_time_series ref_time_series

%% 2) apply normalized window

if user_window_args == true   % make the window using user's options
    if debugging == true
        disp('using user window args')
        disp(varargin(:))
    end

    % make the window
    win = window(win_pointer, orig_points, varargin{:});

else                          % make the window using default or preset
values

    if strcmp(func2str(win_pointer), 'hann')  % replaces strcmp(win_pointer,
'@hann')
```

```
        win_args = true;    % are there any arguments?
        win_opts = 'periodic';
    else
        win_args = false;
        win_opts = [];
    end

    if win_args == true
        win = window(win_pointer, orig_points, win_opts);
    else
        win = window(win_pointer, orig_points);
    end
end    % end basic window constuction

win_norm = sqrt(1/mean(win.^2));
win = win * win_norm;

detrended_windowed_data1 = win .* detrended_data1;

detrend_win_ref = zeros(size(detrend_ref));
for ii = 1:ref_chans  % detrend each ref channel
    detrend_win_ref(:,ii) = win .* detrend_ref(:,ii);
end

%detrended_windowed_data2 = win .* detrended_data2;

if debugging == true
    figure
    pp = plot(time, detrended_data1, 'b', time, detrended_windowed_data1,
'm');
    set(pp,'LineWidth',2)
    title('detrended data 1 vs. windowed, detrended data 1')
    xlabel('time (sec)')
    ylabel('mag')
    legend('detrended data','windowed and detrended data')
    grid on


    set(pp,'LineWidth',2)
    title('detrended data 2 vs. windowed, detrended data 2')
    xlabel('time (sec)')
    ylabel('mag')
    legend('detrended data','windowed and detrended data')
    grid on
    FillPage('t')
    IDfig
    figure
    for ii = 1:ref_chans
        subplot(ref_chans,1,ii)
        pp = plot(time, detrend_ref(:,ii), 'b', ...
            time, detrend_win_ref(:,ii), 'm');
        set(pp,'LineWidth',2)
        title(['Detrended vs. Windowed and detrended, chan ',num2str(ii)])
        xlabel('time (sec)')
        ylabel('mag')
```

```
        legend('detrended data','windowed and detrended')
        grid on
        FillPage('t')
        IDfig
    end

    pow_detrend_series1 = mean(detrended_data1.^2);
    pow_win_detrend_series1 = mean(detrended_windowed_data1.^2);
    pow_detrend_series2 = mean(detrend_ref.^2,1);
    pow_win_detrend_series2 = mean(detrend_win_ref.^2,1);

    disp('avg power:')
    disp(['series 1, before win = ',num2str(pow_detrend_series1)]);
    disp(['series 1, after win = ',num2str(pow_win_detrend_series1)]);
    disp(' ')
    disp(['ref series, before win = ',num2str(pow_detrend_series2)]);
    disp(['ref series, after win = ',num2str(pow_win_detrend_series2)]);
end

clear time win detrended_data1 detrend_ref;

%% 3) calc the ffts
% X is the signal, Y is the ref.
fX_big          = fft(detrended_windowed_data1);
old_fft_points  = ceil(length(fX_big)/2);
data_sig_f      = fX_big(1:old_fft_points);
clear fX_big

% take the fft along each column
% column is the default, but I put in 1 for dim just to be explicit.
%( and guard against matlab updates) - BTL
fY_big     = fft(detrend_win_ref,[],1);
data_ref_f = fY_big(1:old_fft_points,:);
clear fY_big

N  = orig_points;
BW = 1/(orig_points*Ts);    % BW of the original series.

full_freq = (0:old_fft_points-1)*BW;




%% 3)averaging - use the 'constant frequency vector method

% copy from specExplain:

%try to explain the fft of a signal by linear combination of reference
channels in frequency bins.
%input:
%data_sig_f: the signal to be explained by other channels, must be one
dimensional colomn vector.
%data_ref_f: the reference channels, must has the same number of rows as the
signal channel.
%bin_size:number of frequency points in each frequency bin.
```

```
%num_bin:total number of bins to be calculated.
%freq:frequency vector of data,must have same size as data_f_sig
%output:
%sig_asd the asd of the data_f_sig in frequency bins, in unit of one/sqrt(Hz)
%noise_asd the asd of the signal that CANNOT be explained by the signal of
ref channels.
%cor the coherence of the signal and the ref channels, which is defined as 1-
(noise_asd.^2)/(noise_asd.^2)
%freq_bin the average frequency of each bin.
%***************** asd of a bin is defined as**********************
%asd(x)=sqrt(x'*x); where x is the vector of singal points inside the bin.
%
% mod by BTL on June 28, 2009 to make the arguments of the zeros into
% vectors. (they were zeros(num_bin,1), now they are zeros([num_bin,1])
% and made num_bin into an integer with floor

% let W = smooth_width, which is odd.
% the DC term will be W wide, for a 2 sided FFT,
% centered about DC term, ie
% let edge = (W-1)/2, the DC goes from -edge -> + edge (for 2 sided ASD)
% or DC -> +edge (for our single sided ASD)
% f(DC:edge)                -> F(DC)
% f(edge+1)..f(edge+width)  -> F(2)
%
% so the number of new points is
% 1 (for the DC term) + floor((old_fft_points - 1(for the DC term))/width)
edge = (smooth_width-1)/2 + 1;  % plus 1 because DC term is element 1;

% first bucket goes from 1...edge.
% second goes from edge+1 ... edge+smooth_width,
% third is edge + 1 + smooth_width ... edge + 2*smooth_width
% Nth goes from edge + 1 +(N-2)*smooth_width ... edge + (N-1) *smooth_width
% or edge + (1:smooth_width) + (N-2)*smooth_width.

new_fft_points    = 1 + floor((old_fft_points-edge)/smooth_width);

% note - the floor() ensures the averaging matrix is rectangular
% or that the number of points in each bucket are the same.
% We will probably not use a few high freq
% points from the original full_fft.

%last_point_to_use = edge + (new_fft_points-1) * smooth_width;

if (edge + smooth_width) > old_fft_points
    error('your smooth_width is too large (or you data is too short)')
end



bin_bandWidth = smooth_width * BW;

resid_asd     = zeros([new_fft_points,1]);
sig_asd       = zeros([new_fft_points,1]);
fit_vect      = zeros([new_fft_points,ref_chans]);
cor           = zeros([new_fft_points,1]);
```

```
% we leave the first bin at 0
% this bin is like a closet,
% it is filled with the skeletons of polyfit removal and windows.

for ii=2:new_fft_points
    %the index of the bin
    index     = edge + (1:smooth_width) + (ii-2)*smooth_width;
    %power of m channel
    pwr       = data_sig_f(index)'*data_sig_f(index);
    %fit m channel to linear combination of ground STS. fit_all is the
coefficient vector.
    fit_all   = data_ref_f(index,:)\data_sig_f(index);

    %calculate residue error.
    err_r     = data_sig_f(index) - data_ref_f(index,:)*fit_all;
    %total error power in the bin.
    err_p     = err_r'*err_r;
    %coherence.
    cor(ii)   = 1-(err_p)/pwr;
    %asp error
    resid_asd(ii) = (sqrt(2)/N) * abs(sqrt(err_p))/sqrt(bin_bandWidth);
    sig_asd(ii)   = (sqrt(2)/N) * abs(sqrt(pwr))  /sqrt(bin_bandWidth);
    fit_vect(ii,:)  = fit_all.';

end

% 3b and 4:
%
% calculate the statistical correction factor for the noise
% see pg 104 of Hua's thesis.
% this arises because any two vectors statistically have some overlap

SCF       = sqrt(1-ref_chans/smooth_width);
resid_asd = resid_asd / SCF;
%
%
dF   = full_freq(smooth_width+1);  % plus 1 because freq vector, DC is term 1
freq = dF * (0:(new_fft_points-1));


end
```
